# Supplementary material for: Physics-Infused Fuzzy Generative Adversarial Network for Robust Failure Prognosis
Source: arXiv:2206.07762 source file (2022-06-15)
Supplement: Supplementary file 1 [file appendix.tex]

The hyperparameters and model structure are provided in Table \ref{tab:bearingCGAN}.

\begin{table}[H]
    \centering
    \begin{tabular}{|c|c|c|}
          \hline     
          Hyperparameter & Generator & Discriminator  \\
        \hline
        Activation & elu & elu \\
        \hline
        Learning Rate & 0.001 & 0.001  \\
        \hline
        Learning Decay & 0.001 & 0.001 \\
        \hline
        Optimizer & Adam & Adam \\
        \hline
        Noise Input Size & 1 & Not Applicable \\
        \hline
         Number of Layers (before concat.) & 5 & 5\\
        \hline
         Type of Layers (before concat.) & Conv-Conv-Conv-Conv-FC & Conv-Conv-Conv-Conv-FC\\
        \hline
        Size of FC Layers (before concat.) & 100 & 100 \\
         \hline
        Number of Layers (after concat.) & 7 & 6 \\
        \hline
        Size of Layers (after concat.) & 100, 75, 75, 75, 75, 50, 40 & 50, 50, 50, 50, 25, 1 \\
         \hline
        Number of Epochs & 100 & 100 \\
        \hline
        Batch Size & 100 & 100 \\
        \hline
        Weight Initialization & He Normal & He Normal\\
        \hline
    \end{tabular}
    \caption{Bearing}
    \label{tab:bearingCGAN}
\end{table}

FC stands for fully connected layer and the conv layer are 2-dimensional convolutions. The convolution layers have the hyperparameters shown in table \ref{tab:BearingConv}. The output of the generator (40) is hyperparameter to tune to modify the amount of abstract features identified and fed into the fuzzy logic model.

\begin{table}[H]
    \centering
    \begin{tabular}{|c|c|c|c|c|c|}
    \hline
      Layer  & Input Channel & Output Channel & Kernel &  Stride & Padding   \\
      \hline
        Convolution 1 & 4 & 32 & 5 & 2 & 0 \\
        \hline
        Convolution 2 & 32 & 32 & 5 & 2 & 0 \\
        \hline
        Convolution 3 & 32 & 16 & 5 & (2,3) & 0 \\
        \hline
        Convolution 4 & 16 & 2 & 5 & (2,3) & 0 \\
        \hline
    \end{tabular}
    \caption{Bearing: Convolution Layers}
    \label{tab:BearingConv}
\end{table}

The hyperparameters and model structure are provided in table \ref{tab:CMAPSSCGAN}.

\begin{table}[H]
    \centering
        \begin{adjustbox}{width=\columnwidth,center}
    \begin{tabular}{|c|c|c|}
        \hline       
        Activation & elu & elu \\
        \hline
        Learning Rate & 0.001 & 0.001  \\
        \hline
        Learning Decay & 0.001 & 0 \\
        \hline
        Optimizer & Adam & Adam \\
        \hline
        Noise Input Size & 1 & Not Applicable \\
        \hline
         Number of Layers (before concat.) & 7 & 7\\
        \hline
         Type of Layers (before concat.) & Conv-MP-Conv-MP-Conv-MP-FC & Conv-MP-Conv-MP-Conv-MP-FC\\
        \hline
        Size of FC Layers (before concat.) & 100 & 100 \\
         \hline
        Number of Layers (after concat.) & 7 & 6 \\
        \hline
        Size of Layers (after concat.) & 100, 75, 75, 75, 75, 50, 10 & 50, 50, 50, 50, 25, 1 \\
         \hline
        Number of Epochs & 500 & 500 \\
        \hline
        Batch Size & 100 & 100 \\
        \hline
        Weight Initialization & He Normal & He Normal\\
        \hline
    \end{tabular}
        \end{adjustbox}
    \caption{C-MAPSS}
    \label{tab:CMAPSSCGAN}
\end{table}

MP stands for max pooling layer and FC stands for fully connected layer. The convolution layers are 1-dimensional convolutions. The max pooling layers all have a kernel of 2 and the convolution layers have the hyperparameters shown in table \ref{tab:CMAPSSConv}. The output of the generator (10) is hyperparameter to tune to modify the amount of abstract features identified and fed into the fuzzy logic model.

\begin{table}[H]
    \centering
    \begin{tabular}{|c|c|c|c|c|c|}
    \hline
      Layer  & Input Channel & Output Channel & Kernel &  Stride & Padding   \\
      \hline
        Convolution 1 & 26 & 4 & 3 & 2 & 0 \\
        \hline
        Convolution 2 & 4 & 2 & 3 & 2 & 0 \\
        \hline
        Convolution 3 & 2 & 2 & 3 & 2 & 0 \\
        \hline
    \end{tabular}
    \caption{C-MAPSS: Convolution Layers}
    \label{tab:CMAPSSConv}
\end{table}
